# Supplementary material for: GroundLink: A Dataset Unifying Human Body Movement and Ground Reaction Dynamics
Source: arXiv:2310.03930 source file (2023-10-05)
Supplement: Supplementary file 1 [file appendix.tex]

\appendix

\section{Motion Capture Marker List}
